# Supplementary material for: Seeing or Guessing? An Empirical Study of Spatial Bias in Vision-Language Models via Counterfactuals
Source: arXiv:2611.38120 source file (2026-11-27)
Supplement: Supplementary file 1 [file appendix_compute.tex]

% ============================================================================
% GENERATED by appendix_more_results/make_more_results_tables.py
%   generated: 2026-09-25 05:57 UTC
%   source   : results.json through eval_v2.summarize (authoritative)
%   DO NOT EDIT BY HAND -- rerun the script instead.
% ============================================================================

\begin{table}[t]
\centering
\caption{\textbf{Compute budget of the main experiments.} Local inference time is the sum of the per-call \texttt{elapsed\_seconds} stored in the runs, converted to GPU-hours with one GPU per call (two for the sharded Qwen3-VL-32B job); API models consume no local GPU and only their call count is listed. The diagnostic sweep is a separate 1254-pair forward+backward pass on Qwen3-VL-8B, sharded over 2 GPUs (\emph{diagnosis/out/full\_run\_*.txt}).}
\label{tab:app_compute}
\small
\begin{tabular}{lccc}
\toprule
\textbf{Phase} & \textbf{Local calls} & \textbf{GPU-hours} & \textbf{API calls} \\
\midrule
Main evaluation (A0) & 41,382 & 20.3 & 22,572 \\
Ablation A (presentation) & 67,716 & 91.7 & 22,572 \\
Ablation B (image content) & 135,432 & 26.4 & 45,144 \\
\midrule
\textbf{Total (measured)} & 244,530 & 138.3 & 90,288 \\
\textbf{Diagnostic sweep} & 3{,}762 & 5.3 & --- \\

\bottomrule
\end{tabular}
\end{table}
