# Supplementary material for: Seeing or Guessing? An Empirical Study of Spatial Bias in Vision-Language Models via Counterfactuals
Source: arXiv:2611.38120 source file (2026-11-27)
Supplement: Supplementary file 2 [file appendix_filtering.tex]

% ============================================================================
% GENERATED by comparison/make_appendix_tables.py -- do not edit by hand.
%   source: rotation_analysis.json / filter_ablation.json / shared_eligible.json
%          (both produced by eval_v2.summarize on the released results.json files)
% ============================================================================
\begin{table*}[t]
\centering
\caption{\textcolor{black}{\textbf{Effect of the pre-filter: main table (1254 pairs) versus the full pool (1297 pairs).} The 43 excluded pairs were re-run for every model under the configuration recorded for its main-table run; all eleven metrics are recomputed with the same implementation. Values in parentheses are percentage-point changes from the main table for the same model; \textcolor{red}{red} = increase, \textcolor{green!60!black}{green} = decrease. 
% $\mathrm{BR}$ changes by at most 0.6pp and never rises by more than 0.08pp.
}}
\label{tab:app_filtering}
\small
\resizebox{\textwidth}{!}{
\begin{tabular}{lccccccc}
\toprule
\textbf{Model} & $\mathbf{Acc^{O}}\uparrow$ & $\mathbf{Acc^{CF}}\uparrow$ & $\mathbf{pAcc}\uparrow$ & $\mathbf{PRR}\downarrow$ & $\mathbf{LBR}\downarrow$ & $\mathbf{BR}\downarrow$ & $\mathbf{CER}\downarrow$ \\
\midrule
\multicolumn{8}{l}{\textit{Closed-source API}} 
\\
\midrule
GPT-5.6 Luna & 0.710 {\scriptsize \textcolor{green!60!black}{($\mathbf{-1.6}$)}} & 0.488 {\scriptsize \textcolor{red}{($\mathbf{+1.2}$)}} & 0.313 {\scriptsize \textcolor{green!60!black}{($\mathbf{-0.4}$)}} & 0.481 {\scriptsize \textcolor{green!60!black}{($\mathbf{-0.3}$)}} & 0.382 {\scriptsize \textcolor{green!60!black}{($\mathbf{-0.2}$)}} & 0.505 {\scriptsize \textcolor{green!60!black}{($\mathbf{-0.3}$)}} & 0.559 {\scriptsize \textcolor{green!60!black}{($\mathbf{-0.4}$)}} \\
GPT-5.6 Terra & 0.756 {\scriptsize \textcolor{green!60!black}{($\mathbf{-1.7}$)}} & 0.404 {\scriptsize \textcolor{red}{($\mathbf{+1.4}$)}} & 0.295 {\scriptsize \textcolor{green!60!black}{($\mathbf{-0.5}$)}} & 0.544 {\scriptsize \textcolor{green!60!black}{($\mathbf{-0.3}$)}} & 0.479 {\scriptsize \textcolor{green!60!black}{($\mathbf{-0.3}$)}} & 0.566 {\scriptsize \textcolor{green!60!black}{($\mathbf{-0.3}$)}} & 0.611 {\scriptsize \textcolor{green!60!black}{($\mathbf{-0.2}$)}} \\
Claude Sonnet 5 & 0.674 {\scriptsize \textcolor{green!60!black}{($\mathbf{-1.5}$)}} & 0.291 {\scriptsize \textcolor{red}{($\mathbf{+1.3}$)}} & 0.140 {\scriptsize \textcolor{green!60!black}{($\mathbf{-0.2}$)}} & 0.725 {\scriptsize \textcolor{green!60!black}{($\mathbf{-0.1}$)}} & 0.638 {\scriptsize \textcolor{green!60!black}{($\mathbf{-0.2}$)}} & 0.735 {\scriptsize \textcolor{green!60!black}{($\mathbf{-0.2}$)}} & 0.794 {\scriptsize \textcolor{green!60!black}{($\mathbf{-0.2}$)}} \\
Claude Opus 5 & 0.644 {\scriptsize \textcolor{green!60!black}{($\mathbf{-1.3}$)}} & 0.300 {\scriptsize \textcolor{red}{($\mathbf{+1.6}$)}} & 0.133 {\scriptsize \textcolor{red}{($\mathbf{+0.1}$)}} & 0.729 {\scriptsize \textcolor{green!60!black}{($\mathbf{-0.5}$)}} & 0.630 {\scriptsize \textcolor{green!60!black}{($\mathbf{-0.4}$)}} & 0.742 {\scriptsize \textcolor{green!60!black}{($\mathbf{-0.5}$)}} & 0.795 {\scriptsize \textcolor{green!60!black}{($\mathbf{-0.6}$)}} \\
Gemini 3.5 Flash Lite & 0.700 {\scriptsize \textcolor{green!60!black}{($\mathbf{-1.6}$)}} & 0.375 {\scriptsize \textcolor{red}{($\mathbf{+1.3}$)}} & 0.237 {\scriptsize \textcolor{green!60!black}{($\mathbf{-0.4}$)}} & 0.584 {\scriptsize \textcolor{green!60!black}{($\mathbf{-0.1}$)}} & 0.514 {\scriptsize \textcolor{green!60!black}{($\mathbf{-0.1}$)}} & 0.603 {\scriptsize \textcolor{green!60!black}{($\mathbf{-0.1}$)}} & 0.663 {\scriptsize \textcolor{green!60!black}{($\mathbf{-0.2}$)}} \\
Gemini 3.8 Flash & 0.756 {\scriptsize \textcolor{green!60!black}{($\mathbf{-1.2}$)}} & 0.490 {\scriptsize \textcolor{red}{($\mathbf{+1.2}$)}} & 0.372 {\scriptsize \textcolor{green!60!black}{($\mathbf{-0.2}$)}} & 0.448 {\scriptsize \textcolor{green!60!black}{($\mathbf{-0.4}$)}} & 0.357 {\scriptsize \textcolor{green!60!black}{($\mathbf{-0.2}$)}} & 0.450 {\scriptsize \textcolor{green!60!black}{($\mathbf{-0.4}$)}} & 0.509 {\scriptsize \textcolor{green!60!black}{($\mathbf{-0.5}$)}} \\
\midrule
\multicolumn{8}{l}{\textit{Open-source local}} \\
\midrule
Qwen3-VL-2B & 0.495 {\scriptsize \textcolor{green!60!black}{($\mathbf{-0.9}$)}} & 0.333 {\scriptsize \textcolor{red}{($\mathbf{+1.1}$)}} & 0.102 {\scriptsize \textcolor{green!60!black}{($\mathbf{-0.0}$)}} & 0.720 {\scriptsize \textcolor{green!60!black}{($\mathbf{-0.3}$)}} & 0.528 {\scriptsize \textcolor{green!60!black}{($\mathbf{-0.2}$)}} & 0.749 {\scriptsize \textcolor{green!60!black}{($\mathbf{-0.2}$)}} & 0.794 {\scriptsize \textcolor{green!60!black}{($\mathbf{-0.3}$)}} \\
Qwen3-VL-8B & 0.665 {\scriptsize \textcolor{green!60!black}{($\mathbf{-1.4}$)}} & 0.283 {\scriptsize \textcolor{red}{($\mathbf{+1.7}$)}} & 0.154 {\scriptsize \textcolor{green!60!black}{($\mathbf{-0.1}$)}} & 0.721 {\scriptsize \textcolor{green!60!black}{($\mathbf{-0.3}$)}} & 0.602 {\scriptsize \textcolor{green!60!black}{($\mathbf{-0.2}$)}} & 0.728 {\scriptsize \textcolor{green!60!black}{($\mathbf{-0.3}$)}} & 0.770 {\scriptsize \textcolor{green!60!black}{($\mathbf{-0.3}$)}} \\
Qwen3-VL-32B & 0.673 {\scriptsize \textcolor{green!60!black}{($\mathbf{-1.8}$)}} & 0.347 {\scriptsize \textcolor{red}{($\mathbf{+1.9}$)}} & 0.196 {\scriptsize \textcolor{green!60!black}{($\mathbf{-0.4}$)}} & 0.637 {\scriptsize \textcolor{green!60!black}{($\mathbf{-0.3}$)}} & 0.550 {\scriptsize \textcolor{green!60!black}{($\mathbf{-0.2}$)}} & 0.665 {\scriptsize \textcolor{green!60!black}{($\mathbf{-0.2}$)}} & 0.709 {\scriptsize \textcolor{green!60!black}{($\mathbf{-0.2}$)}} \\
InternVL3.5-2B & 0.554 {\scriptsize \textcolor{green!60!black}{($\mathbf{-0.8}$)}} & 0.256 {\scriptsize \textcolor{red}{($\mathbf{+1.4}$)}} & 0.064 {\scriptsize \textcolor{red}{($\mathbf{+0.0}$)}} & 0.821 {\scriptsize \textcolor{green!60!black}{($\mathbf{-0.2}$)}} & 0.644 {\scriptsize \textcolor{red}{($\mathbf{+0.1}$)}} & 0.844 {\scriptsize \textcolor{green!60!black}{($\mathbf{-0.3}$)}} & 0.886 {\scriptsize \textcolor{green!60!black}{($\mathbf{-0.2}$)}} \\
InternVL3.5-8B & 0.523 {\scriptsize \textcolor{green!60!black}{($\mathbf{-0.7}$)}} & 0.284 {\scriptsize \textcolor{red}{($\mathbf{+0.8}$)}} & 0.081 {\scriptsize \textcolor{green!60!black}{($\mathbf{-0.0}$)}} & 0.781 {\scriptsize \textcolor{red}{($\mathbf{+0.0}$)}} & 0.639 {\scriptsize \textcolor{green!60!black}{($\mathbf{-0.3}$)}} & 0.818 {\scriptsize \textcolor{green!60!black}{($\mathbf{-0.1}$)}} & 0.847 {\scriptsize \textcolor{green!60!black}{($\mathbf{-0.1}$)}} \\
InternVL3.5-14B & 0.607 {\scriptsize \textcolor{green!60!black}{($\mathbf{-1.5}$)}} & 0.292 {\scriptsize \textcolor{red}{($\mathbf{+1.6}$)}} & 0.108 {\scriptsize \textcolor{green!60!black}{($\mathbf{-0.1}$)}} & 0.763 {\scriptsize \textcolor{green!60!black}{($\mathbf{-0.3}$)}} & 0.619 {\scriptsize \textcolor{green!60!black}{($\mathbf{-0.2}$)}} & 0.785 {\scriptsize \textcolor{green!60!black}{($\mathbf{-0.3}$)}} & 0.823 {\scriptsize \textcolor{green!60!black}{($\mathbf{-0.4}$)}} \\
LLaVA-1.5-7B & 0.479 {\scriptsize \textcolor{green!60!black}{($\mathbf{-0.0}$)}} & 0.288 {\scriptsize \textcolor{red}{($\mathbf{+0.0}$)}} & 0.027 {\scriptsize \textcolor{green!60!black}{($\mathbf{-0.0}$)}} & 0.912 {\scriptsize \textcolor{green!60!black}{($\mathbf{-0.0}$)}} & 0.554 {\scriptsize \textcolor{green!60!black}{($\mathbf{-0.5}$)}} & 0.928 {\scriptsize \textcolor{green!60!black}{($\mathbf{-0.1}$)}} & 0.943 {\scriptsize \textcolor{red}{($\mathbf{+0.0}$)}} \\
MiniCPM-V 4.6 & 0.487 {\scriptsize \textcolor{green!60!black}{($\mathbf{-0.9}$)}} & 0.354 {\scriptsize \textcolor{red}{($\mathbf{+0.7}$)}} & 0.111 {\scriptsize \textcolor{green!60!black}{($\mathbf{-0.2}$)}} & 0.686 {\scriptsize \textcolor{red}{($\mathbf{+0.1}$)}} & 0.507 {\scriptsize \textcolor{red}{($\mathbf{+0.1}$)}} & 0.720 {\scriptsize \textcolor{red}{($\mathbf{+0.1}$)}} & 0.775 {\scriptsize \textcolor{red}{($\mathbf{+0.0}$)}} \\
GLM-4.1V-9B & 0.695 {\scriptsize \textcolor{green!60!black}{($\mathbf{-1.4}$)}} & 0.315 {\scriptsize \textcolor{red}{($\mathbf{+1.4}$)}} & 0.187 {\scriptsize \textcolor{green!60!black}{($\mathbf{-0.2}$)}} & 0.673 {\scriptsize \textcolor{green!60!black}{($\mathbf{-0.2}$)}} & 0.579 {\scriptsize \textcolor{green!60!black}{($\mathbf{-0.5}$)}} & 0.694 {\scriptsize \textcolor{green!60!black}{($\mathbf{-0.3}$)}} & 0.734 {\scriptsize \textcolor{green!60!black}{($\mathbf{-0.3}$)}} \\
\midrule
\multicolumn{8}{l}{\textit{Spatially specialised}} \\
\midrule
SpatioLM-Understanding & 0.511 {\scriptsize \textcolor{green!60!black}{($\mathbf{-1.1}$)}} & 0.235 {\scriptsize \textcolor{red}{($\mathbf{+1.0}$)}} & 0.079 {\scriptsize \textcolor{red}{($\mathbf{+0.0}$)}} & 0.754 {\scriptsize \textcolor{green!60!black}{($\mathbf{-0.3}$)}} & 0.623 {\scriptsize \textcolor{green!60!black}{($\mathbf{-0.3}$)}} & 0.793 {\scriptsize \textcolor{green!60!black}{($\mathbf{-0.4}$)}} & 0.848 {\scriptsize \textcolor{green!60!black}{($\mathbf{-0.4}$)}} \\
SpatialRGPT-8B & 0.472 {\scriptsize \textcolor{green!60!black}{($\mathbf{-0.4}$)}} & 0.248 {\scriptsize \textcolor{red}{($\mathbf{+1.0}$)}} & 0.040 {\scriptsize \textcolor{red}{($\mathbf{+0.0}$)}} & 0.853 {\scriptsize \textcolor{red}{($\mathbf{+0.0}$)}} & 0.716 {\scriptsize \textcolor{green!60!black}{($\mathbf{-0.1}$)}} & 0.892 {\scriptsize \textcolor{green!60!black}{($\mathbf{-0.1}$)}} & 0.917 {\scriptsize \textcolor{green!60!black}{($\mathbf{-0.1}$)}} \\
\bottomrule
\end{tabular}
}
\end{table*}
