# Supplementary material for: Seeing or Guessing? An Empirical Study of Spatial Bias in Vision-Language Models via Counterfactuals
Source: arXiv:2611.38120 source file (2026-11-27)
Supplement: Supplementary file 3 [file appendix_shared_eligible.tex]

% ============================================================================
% GENERATED by comparison/make_appendix_tables.py -- do not edit by hand.
%   source: rotation_analysis.json / filter_ablation.json / shared_eligible.json
%          (both produced by eval_v2.summarize on the released results.json files)
% ============================================================================
\begin{table*}[t]
\centering
\caption{\textbf{Comparison on a fixed population.} Each model's $\mathrm{BR}$ is defined on its own eligible set $E_M$; here every metric is recomputed on the intersection $\cap_M E_M$, which contains 58 pairs. On the intersection the original-image question is answered correctly by construction, so $Acc^{O}=1$ and only the counterfactual side informs. Ranks are over the 17 models, with the shift from the own-set ranking in parentheses; \textcolor{red}{red} = the model looks worse on the fixed population.}
\label{tab:app_shared_eligible}
\small
\resizebox{\textwidth}{!}{
\begin{tabular}{lcccccccc}
\toprule
\textbf{Model} & $\mathbf{n_{E_M}}$ & $\mathbf{BR}$ (own) & $\mathbf{BR}$ (shared) & $\mathbf{\Delta BR}$ &
$\mathbf{Acc^{CF}}$ (own) & $\mathbf{Acc^{CF}}$ (shared) & \textbf{rank (own)} & \textbf{rank (shared)} \\
\midrule
Gemini 3.8 Flash & 939 & 0.450 & 0.448 & {\scriptsize \textcolor{green!60!black}{($\mathbf{-0.2}$)}} & 0.490 & 0.483 & 1 & 1 \\
GPT-5.6 Luna & 888 & 0.505 & 0.569 & {\scriptsize \textcolor{red}{($\mathbf{+6.4}$)}} & 0.488 & 0.379 & 2 & 3 {\scriptsize \textcolor{red}{(+1)}} \\
GPT-5.6 Terra & 945 & 0.566 & 0.690 & {\scriptsize \textcolor{red}{($\mathbf{+12.4}$)}} & 0.404 & 0.293 & 3 & 10 {\scriptsize \textcolor{red}{(+7)}} \\
Gemini 3.5 Flash Lite & 876 & 0.603 & 0.500 & {\scriptsize \textcolor{green!60!black}{($\mathbf{-10.3}$)}} & 0.375 & 0.414 & 4 & 2 {\scriptsize \textcolor{green!60!black}{(-2)}} \\
Qwen3-VL-32B & 842 & 0.665 & 0.655 & {\scriptsize \textcolor{green!60!black}{($\mathbf{-1.0}$)}} & 0.347 & 0.276 & 5 & 8 {\scriptsize \textcolor{red}{(+3)}} \\
GLM-4.1V-9B & 860 & 0.694 & 0.638 & {\scriptsize \textcolor{green!60!black}{($\mathbf{-5.6}$)}} & 0.315 & 0.293 & 6 & 6 \\
MiniCPM-V 4.6 & 608 & 0.720 & 0.621 & {\scriptsize \textcolor{green!60!black}{($\mathbf{-10.0}$)}} & 0.354 & 0.328 & 7 & 4 {\scriptsize \textcolor{green!60!black}{(-3)}} \\
Qwen3-VL-8B & 832 & 0.728 & 0.621 & {\scriptsize \textcolor{green!60!black}{($\mathbf{-10.8}$)}} & 0.283 & 0.293 & 8 & 5 {\scriptsize \textcolor{green!60!black}{(-3)}} \\
Claude Sonnet 5 & 843 & 0.735 & 0.707 & {\scriptsize \textcolor{green!60!black}{($\mathbf{-2.9}$)}} & 0.291 & 0.172 & 9 & 11 {\scriptsize \textcolor{red}{(+2)}} \\
Claude Opus 5 & 805 & 0.742 & 0.690 & {\scriptsize \textcolor{green!60!black}{($\mathbf{-5.2}$)}} & 0.300 & 0.190 & 10 & 9 {\scriptsize \textcolor{green!60!black}{(-1)}} \\
Qwen3-VL-2B & 621 & 0.749 & 0.638 & {\scriptsize \textcolor{green!60!black}{($\mathbf{-11.1}$)}} & 0.333 & 0.276 & 11 & 7 {\scriptsize \textcolor{green!60!black}{(-4)}} \\
InternVL3.5-14B & 759 & 0.785 & 0.724 & {\scriptsize \textcolor{green!60!black}{($\mathbf{-6.1}$)}} & 0.292 & 0.241 & 12 & 12 \\
SpatioLM-Understanding & 639 & 0.793 & 0.776 & {\scriptsize \textcolor{green!60!black}{($\mathbf{-1.8}$)}} & 0.235 & 0.155 & 13 & 14 {\scriptsize \textcolor{red}{(+1)}} \\
InternVL3.5-8B & 654 & 0.818 & 0.776 & {\scriptsize \textcolor{green!60!black}{($\mathbf{-4.2}$)}} & 0.284 & 0.155 & 14 & 13 {\scriptsize \textcolor{green!60!black}{(-1)}} \\
InternVL3.5-2B & 694 & 0.844 & 0.793 & {\scriptsize \textcolor{green!60!black}{($\mathbf{-5.1}$)}} & 0.256 & 0.155 & 15 & 15 \\
SpatialRGPT-8B & 591 & 0.892 & 0.845 & {\scriptsize \textcolor{green!60!black}{($\mathbf{-4.7}$)}} & 0.248 & 0.103 & 16 & 16 \\
LLaVA-1.5-7B & 601 & 0.928 & 0.879 & {\scriptsize \textcolor{green!60!black}{($\mathbf{-4.9}$)}} & 0.288 & 0.103 & 17 & 17 \\
\bottomrule
\end{tabular}
}
\end{table*}
